# Supplementary material for: uDistil-Whisper: Label-Free Data Filtering for Knowledge Distillation in Low-Data Regimes
Source: arXiv:2407.01257 source file (2025-05-15)
Supplement: Supplementary file 1 [file 10_1_methods_appendix.tex]

% \KK{maybe add smt to introduce the diff methods (ill do it)}

\subsubsection{Proxy Models}
\KKcomment{If we came up with this method and coined this "proxy model" name, I think we should make it clearer by using "we". In this method we use a separate.. that we refer to as proxy model...} This method utilizes a separate, pre-trained ASR model (referred to as proxy model) to generate reference transcripts for the input speech. The quality of the teacher model's pseudo-label is then assessed based on the Word Error Rate between the proxy model's reference and the teacher's reference, \KK{which we call \textit{pWER}}.
Lower \textit{pWER} values indicate better agreement between the teacher and proxy models, suggesting higher confidence and reliability in the pseudo-label. A pre-defined WER threshold can be used to filter out examples exceeding the acceptable error rate. In our work, we use SeamlessM4T-large-v2 \mam{cite this} as our choice of proxy model.

\subsection{Uncertainty Quantification}
We leverage the uncertainty in the teacher's output to filter out low-quality examples. In other words, we employ measures derived from the teacher model's confidence scores to identify pseudo-labels with high reliability. In particular, we we employ the following two commonly used uncertainty metrics:

\noindent\textbf{Entropy.} Entropy measures the information uncertainty associated with the teacher's predicted probability distribution over the vocabulary. High entropy indicates that the model is unsure about the correct word, suggesting a lower confidence in the pseudo-label.
The entropy $H$ for a single utterance with $N$ words is calculated as:

\begin{equation}
H = -\sum_{i=1}^{N} p_i \log_2(p_i)
\end{equation}

\noindent where $p_i$ represents the teacher model's predicted probability for the $i^{\text{th}}$ word in the utterance.

\noindent\textbf{Geometric Mean of Confidence Scores.} This metric calculates the geometric mean of individual confidence scores assigned by the teacher model to each word in the pseudo-label. A high geometric mean suggests that the model is confident about the predicted sequence, implying a more reliable pseudo-label. The geometric mean $G$ of confidence scores for an $N$-word utterance is:

\begin{equation}
G = \sqrt[N]{\prod_{i=1}^{N} c_i}
\end{equation}

\noindent where $c_i$ denotes the confidence score assigned by the teacher model for the $i^{\text{th}}$ word.
During filtering, examples with low entropy and a high geometric mean are considered reliable and are retained for training the student model.

\subsubsection{Negative Log Likelihood}
We make use of an AceGPT-7B~\cite{huang2024acegpt} language model to compute the log-likelihood of the teacher's output. A lower negative log-likelihood indicates higher compatibility between the pseudo-label and the language model's understanding of natural language, suggesting a more accurate pseudo-label.
The negative log-likelihood $NLL$ for a teacher-predicted pseudo-label sequence $y$ of length $T$ is:

\begin{equation}
NLL = -\sum_{t=1}^{T} \log(p(y_t | y_{1...t-1}))
\end{equation}

\noindent where $p(y_t | y_{1...t-1})$ is the probability assigned by the language model to $y_t$, the $t^{\text{th}}$ word in the pseudo-label sequence, given the previous words $(y_{1...t-1})$.
Pseudo labels with lower negative log-likelihood values are preferred, as they are more likely to form coherent sequences in the language model, indicating higher-quality pseudo-labels suitable for training the student models.

\subsubsection{Multimodal Embeddings}
We use SONAR~\cite{duquenne2023sonar} to generate embeddings for both input speech segments and their corresponding pseudo-labels. These embeddings capture the contextual information of the speech signals and the text representations derived from the pseudo-labels. The similarity between these embeddings is computed using the dot product, serving as a measure of how closely aligned the speech and pseudo-label representations are.
A high similarity score indicates strong contextual alignment between the speech and text, suggesting that the pseudo-label accurately reflects the content of the speech segment. This helps in identifying and retaining high-quality pseudo-labels while filtering out those that do not adequately represent the speech content.
%By leveraging the similarity scores derived from SONAR embeddings, we effectively enhance the quality of the pseudo-labels used in training, improving the overall performance as a result. %This method enables more accurate model training in scenarios where labeled data is limited or unavailable, optimizing the efficiency and effectiveness of the learning process.

\subsubsection{Similarity with Synthetic Speech}
In this approach, we start by generating synthetic speech from the pseudo-labels' text using \textit{XTTS-v2}\footnote{\url{https://huggingface.co/coqui/XTTS-v2}}. Next, we compute the similarity between the synthetic speech and the ground truth speech. To assess the quality of the synthetic speech compared to the original speech segment, we utilize metrics such as Perceptual Evaluation of Speech Quality (PESQ) \KKcomment{is there a paper to cite?} and Mel-Cepstral Distortion (MCD) \KKcomment{same?}. A high similarity score suggests that the pseudo-labels are likely to have minimal errors.
When evaluating these metrics in relation to the Word Error Rate (WER), we observe that PESQ shows a stronger correlation. Therefore, we select PESQ as the primary metric for our experiments. %This choice ensures an effective assessment of synthetic speech quality and alignment with the original speech, enhancing the reliability of our pseudo-labeling approach.
